# Supplementary material for: Problems with SZZ and Features: An empirical study of the state of practice of defect prediction data collection
Source: arXiv:1911.08938 source file (2021-11-11)
Supplement: Supplementary file 1 [file supplemental.tex]

\appendix
\section{Supplemental Material}

\begin{table*}
\begin{tabular}{llllllll}
\textbf{Project} & \textbf{Linked Bug Issues} & \textbf{BUG} & \textbf{IMPROVEMENT} & \textbf{TEST} & \textbf{DOCUMENTATION} & \textbf{OTHER} & missing \\
\hline
ant-ivy & 535 & 8 (0.01) & 0 & 0 & 1 & 1 & 525 (0.98) \\
archiva & 542 & 0 (0.00) & 0 & 0 & 0 & 0 & 542 (1.00) \\
calcite & 842 & 0 (0.00) & 0 & 0 & 0 & 0 & 842 (1.00) \\
cayenne & 530 & 0 (0.00) & 0 & 0 & 0 & 0 & 530 (1.00) \\
commons-bcel & 53 & 28 (0.53) & 11 & 0 & 2 & 0 & 12 (0.23) \\
commons-beanutils & 76 & 42 (0.55) & 15 & 0 & 2 & 3 & 14 (0.18) \\
commons-codec & 64 & 27 (0.42) & 14 & 1 & 10 & 1 & 11 (0.17) \\
commons-collections & 115 & 39 (0.34) & 42 & 1 & 13 & 3 & 17 (0.15) \\
commons-compress & 172 & 105 (0.61) & 14 & 1 & 5 & 3 & 44 (0.26) \\
commons-configuration & 188 & 123 (0.65) & 17 & 3 & 5 & 8 & 32 (0.17) \\
commons-dbcp & 127 & 59 (0.46) & 23 & 0 & 3 & 4 & 38 (0.30) \\
commons-digester & 26 & 15 (0.58) & 2 & 0 & 1 & 0 & 8 (0.31) \\
commons-imaging & 42 & 26 (0.62) & 9 & 0 & 0 & 0 & 7 (0.17) \\
commons-io & 131 & 64 (0.49) & 18 & 6 & 13 & 3 & 27 (0.21) \\
commons-jcs & 80 & 54 (0.68) & 11 & 3 & 1 & 2 & 9 (0.11) \\
commons-jexl & 84 & 52 (0.62) & 12 & 1 & 6 & 0 & 13 (0.15) \\
commons-lang & 315 & 0 (0.00) & 0 & 0 & 0 & 0 & 315 (1.00) \\
commons-math & 415 & 238 (0.57) & 119 & 18 & 35 & 4 & 1 (0.00) \\
commons-net & 176 & 127 (0.72) & 36 & 2 & 9 & 0 & 2 (0.01) \\
commons-rdf & 15 & 6 (0.40) & 2 & 1 & 1 & 2 & 3 (0.20) \\
commons-scxml & 70 & 42 (0.60) & 10 & 4 & 1 & 0 & 13 (0.19) \\
commons-validator & 73 & 53 (0.73) & 4 & 1 & 0 & 1 & 14 (0.19) \\
commons-vfs & 156 & 78 (0.50) & 26 & 4 & 6 & 8 & 34 (0.22) \\
deltaspike & 302 & 0 (0.00) & 0 & 0 & 0 & 0 & 302 (1.00) \\
directory-fotress-core & 60 & 0 (0.00) & 0 & 0 & 0 & 0 & 60 (1.00) \\
falcon & 741 & 0 (0.00) & 0 & 0 & 0 & 0 & 741 (1.00) \\
giraph & 336 & 0 (0.00) & 0 & 0 & 0 & 0 & 336 (1.00) \\
gora & 113 & 0 (0.00) & 0 & 0 & 0 & 0 & 113 (1.00) \\
jspwiki & 268 & 0 (0.00) & 0 & 0 & 0 & 0 & 268 (1.00) \\
knox & 566 & 0 (0.00) & 0 & 0 & 0 & 0 & 566 (1.00) \\
kylin & 732 & 0 (0.00) & 0 & 0 & 0 & 0 & 732 (1.00) \\
lens & 396 & 0 (0.00) & 0 & 0 & 0 & 0 & 396 (1.00) \\
mahout & 513 & 0 (0.00) & 0 & 0 & 0 & 0 & 513 (1.00) \\
manifoldcf & 633 & 0 (0.00) & 0 & 0 & 0 & 0 & 633 (1.00) \\
nutch & 643 & 0 (0.00) & 0 & 0 & 0 & 0 & 643 (1.00) \\
opennlp & 219 & 0 (0.00) & 0 & 0 & 0 & 0 & 219 (1.00) \\
parquet-mr & 185 & 0 (0.00) & 0 & 0 & 0 & 0 & 185 (1.00) \\
santuario-java & 83 & 0 (0.00) & 0 & 0 & 0 & 0 & 83 (1.00) \\
systemml & 452 & 0 (0.00) & 0 & 0 & 0 & 0 & 452 (1.00) \\
tika & 605 & 0 (0.00) & 0 & 0 & 0 & 0 & 605 (1.00) \\
wss4j & 241 & 0 (0.00) & 0 & 0 & 0 & 0 & 241 (1.00) \\
xerces2-j & 238 & 0 (0.00) & 0 & 0 & 0 & 0 & 238 (1.00) \\
\hline
Total & 12153 & 1186 (0.10) & 385 & 46 & 114 & 43 & 10379 (0.85) \\
\end{tabular}
\caption{Data about manual issue type validation}
\label{tbl:issue_validation_data}
\end{table*}

\begin{table*}
\begin{tabular}{llllll}
\textbf{Project} & \textbf{Commits} & \textbf{SZZ} & \textbf{JLV} & \textbf{JLVM} \\
\hline
archiva & 10261 & 2021 & 949 & 0 & 0 \\
ant-ivy & 3189 & 796 & 716 & 11 & 0 \\
commons-bcel & 1429 & 85 & 95 & 45 & 0 \\
commons-beanutils & 1341 & 128 & 119 & 56 & 0 \\
commons-codec & 1838 & 153 & 155 & 60 & 0 \\
commons-collections & 3380 & 199 & 180 & 75 & 0 \\
commons-compress & 2755 & 699 & 323 & 212 & 0 \\
commons-configuration & 3717 & 342 & 348 & 224 & 0 \\
commons-dbcp & 2205 & 401 & 192 & 91 & 0 \\
commons-digester & 2535 & 82 & 38 & 24 & 0 \\
commons-imaging & 1066 & 198 & 64 & 27 & 0 \\
commons-io & 2262 & 219 & 245 & 106 & 0 \\
commons-jcs & 1622 & 364 & 161 & 74 & 0 \\
commons-jexl & 3276 & 349 & 258 & 152 & 0 \\
commons-math & 7222 & 736 & 726 & 397 & 396 \\
commons-net & 2270 & 321 & 250 & 174 & 174 \\
commons-rdf & 1311 & 94 & 62 & 30 & 0 \\
commons-scxml & 1216 & 286 & 123 & 60 & 0 \\
commons-validator & 3416 & 182 & 104 & 69 & 0 \\
commons-vfs & 2212 & 225 & 211 & 113 & 0 \\
\hline
Total & 58523 & 7880 & 5319 & 2000 & 570 \\
\end{tabular}
\caption{Data about different strategies to determine bugfixing commits}
\label{tbl:bugfix_validation_data}
\end{table*}
